# Supplementary material for: Learning to Parallelize with OpenMP by Augmented Heterogeneous AST Representation
Source: arXiv:2305.05779 source file (2023-05-09)
Supplement: Supplementary file 1 [file 9-appendix.tex]

\appendix 
\section{Synthetic Dataset Generation} 
\label{app:synthetic}

\subsection{Generating Loops with Do-all Pattern}

Let us consider the template in Listing \ref{ls:jinja1} and the generated code using that template in Listing \ref{ls:jinja1-1}. Here the $counter$ is replaced by variable $o$. We generated the variable names randomly by using a combination of English language alphabets (a-z, A-Z), digits (0-9) and underscore (\_). $limit$ is replaced by an arbitrary integer $246$. In the left side of do-all equation we replace the ${{operand}}$ by one of our randomly generated array variables $s$. In the right side of the do-all equation we can have both variables and constants which are also chosen arbitrarily. For the ${{operator}}$ we consider $+,\ -,\ *,\ /$ operations.

\begin{minipage}[H]{\linewidth}
\begin{lstlisting}[frame=single, caption=A sample template of a loop containing do-all pattern,label=ls:jinja1, captionpos=b, basicstyle=\small, language=C]
  for ({{counter}} = 0; {{counter}} < 
  {{limit}}; {{counter}} = {{counter}} + 
  {{constant}})
  {
      //do-all equation
      {{operand}} = {{operand}}
      {{operator}} {{operand}};
  }
\end{lstlisting}
\end{minipage}

\begin{minipage}[H]{\linewidth}
\begin{lstlisting}[frame=single, caption=A loop containing do-all pattern generated from the template in Listing \ref{ls:jinja1},label=ls:jinja1-1, captionpos=b, basicstyle=\small, language=C]
  for (o = 0; o < 246; o = o + 1)
  {
      s[o] =  j6 + 20;
  }
\end{lstlisting}
\end{minipage}

Listing \ref{ls:jinja3} presents another one of our templates for do-all pattern. Listing \ref{ls:jinja3-1} represents the loop generated from this template.

\begin{minipage}[H]{\linewidth}
\begin{lstlisting}[frame=single, caption=A sample template of a loop containing do-all pattern,label=ls:jinja3, captionpos=b, basicstyle=\small, language=C]
  for ({{counter}} = 0; {{counter}} < 
  {{limit}}; {{counter}} = {{counter}} + 
  {{constant}})
  {
      //do-all equation 2
      {{operand}} = {{operand}};
  }
\end{lstlisting}
\end{minipage}

\begin{minipage}[H]{\linewidth}
\begin{lstlisting}[frame=single, caption=A loop containing do-all pattern generated from the
template in Listing \ref{ls:jinja3},label=ls:jinja3-1, captionpos=b, basicstyle=\small, language=C]
  for (cb1 = 0; cb1 < 33211; cb1 = cb1 + 1)
  {
      ar[cb1] =  _q522;
  }
\end{lstlisting}
\end{minipage}

\subsection{Generating Loops with Reduction Pattern}

Now let us consider the reduction template in Listing \ref{ls:jinja2} and the generated reduction loop in Listing \ref{ls:jinja2-1}. $counter$ and $red\_var$ are replaced using randomly generated variables $n$ and $quC$ respectively. $limit$ and $term$ are replaced by randomly generated integer constants $184$ and $4$ respectively. The reduction operation needs to be associative and commutative so we only considered $+$ and $*$ operation and arbitrarily picked one of them in place of $red\_operator$.

% \vspace{4pt}
\begin{minipage}[H]{\linewidth}
\begin{lstlisting}[frame=single,caption=A sample template of a loop containing reduction pattern,label=ls:jinja2, captionpos=b, basicstyle=\small, language=C]
  for ({{counter}} = 0; {{counter}} < 
  {{limit}}; {{counter}} = {{counter}} +
  {{constant}}) 
  {
      /*reduction equation*/
      {{red_var}} = {{red_var}} 
      {{red_operator}} ({{term}});
  }
\end{lstlisting}
\end{minipage}

\begin{minipage}[H]{\linewidth}
\begin{lstlisting}[frame=single,caption=A loop containing reduction pattern generated from the template in Listing \ref{ls:jinja2},label=ls:jinja2-1, captionpos=b, basicstyle=\small, language=C]
  for (n = 0; n < 184; n = n + 1) {
      quC = quC + 4;
  }
\end{lstlisting}
\end{minipage}

Listing \ref{ls:jinja4} presents another one of our templates for the reduction pattern and listing \ref{ls:jinja4-1} represents the loop generated from this template.

\begin{minipage}[H]{\linewidth}
\begin{lstlisting}[frame=single,caption=A sample template of a loop containing reduction pattern,label=ls:jinja4, captionpos=b, basicstyle=\small, language=C]
  for ({{counter}} = 0; {{counter}} < 
  {{limit}}; {{counter}} = {{counter}} +
  {{constant}}) 
  {
      /*reduction equation 2*/
      {{red_var}} {{red_operator}} =
       ({{term}});
  }
\end{lstlisting}
\end{minipage}

\begin{minipage}[H]{\linewidth}
\begin{lstlisting}[frame=single,caption=A loop containing reduction pattern generated from the template in Listing \ref{ls:jinja2},label=ls:jinja4-1, captionpos=b, basicstyle=\small, language=C]
  for (nd3 = 0; nd3 < 184; nd3 = nd3 + 5) {
      C_2a *= 411;
  }
\end{lstlisting}
\end{minipage}

\section{Evaluation}
Figure \ref{fig:ast_loss}, \ref{fig:acc}, and \ref{fig:acc2} present the training details.
\label{app:eval}
\begin{figure}[h]
    \centering
    \includegraphics[width=8cm]{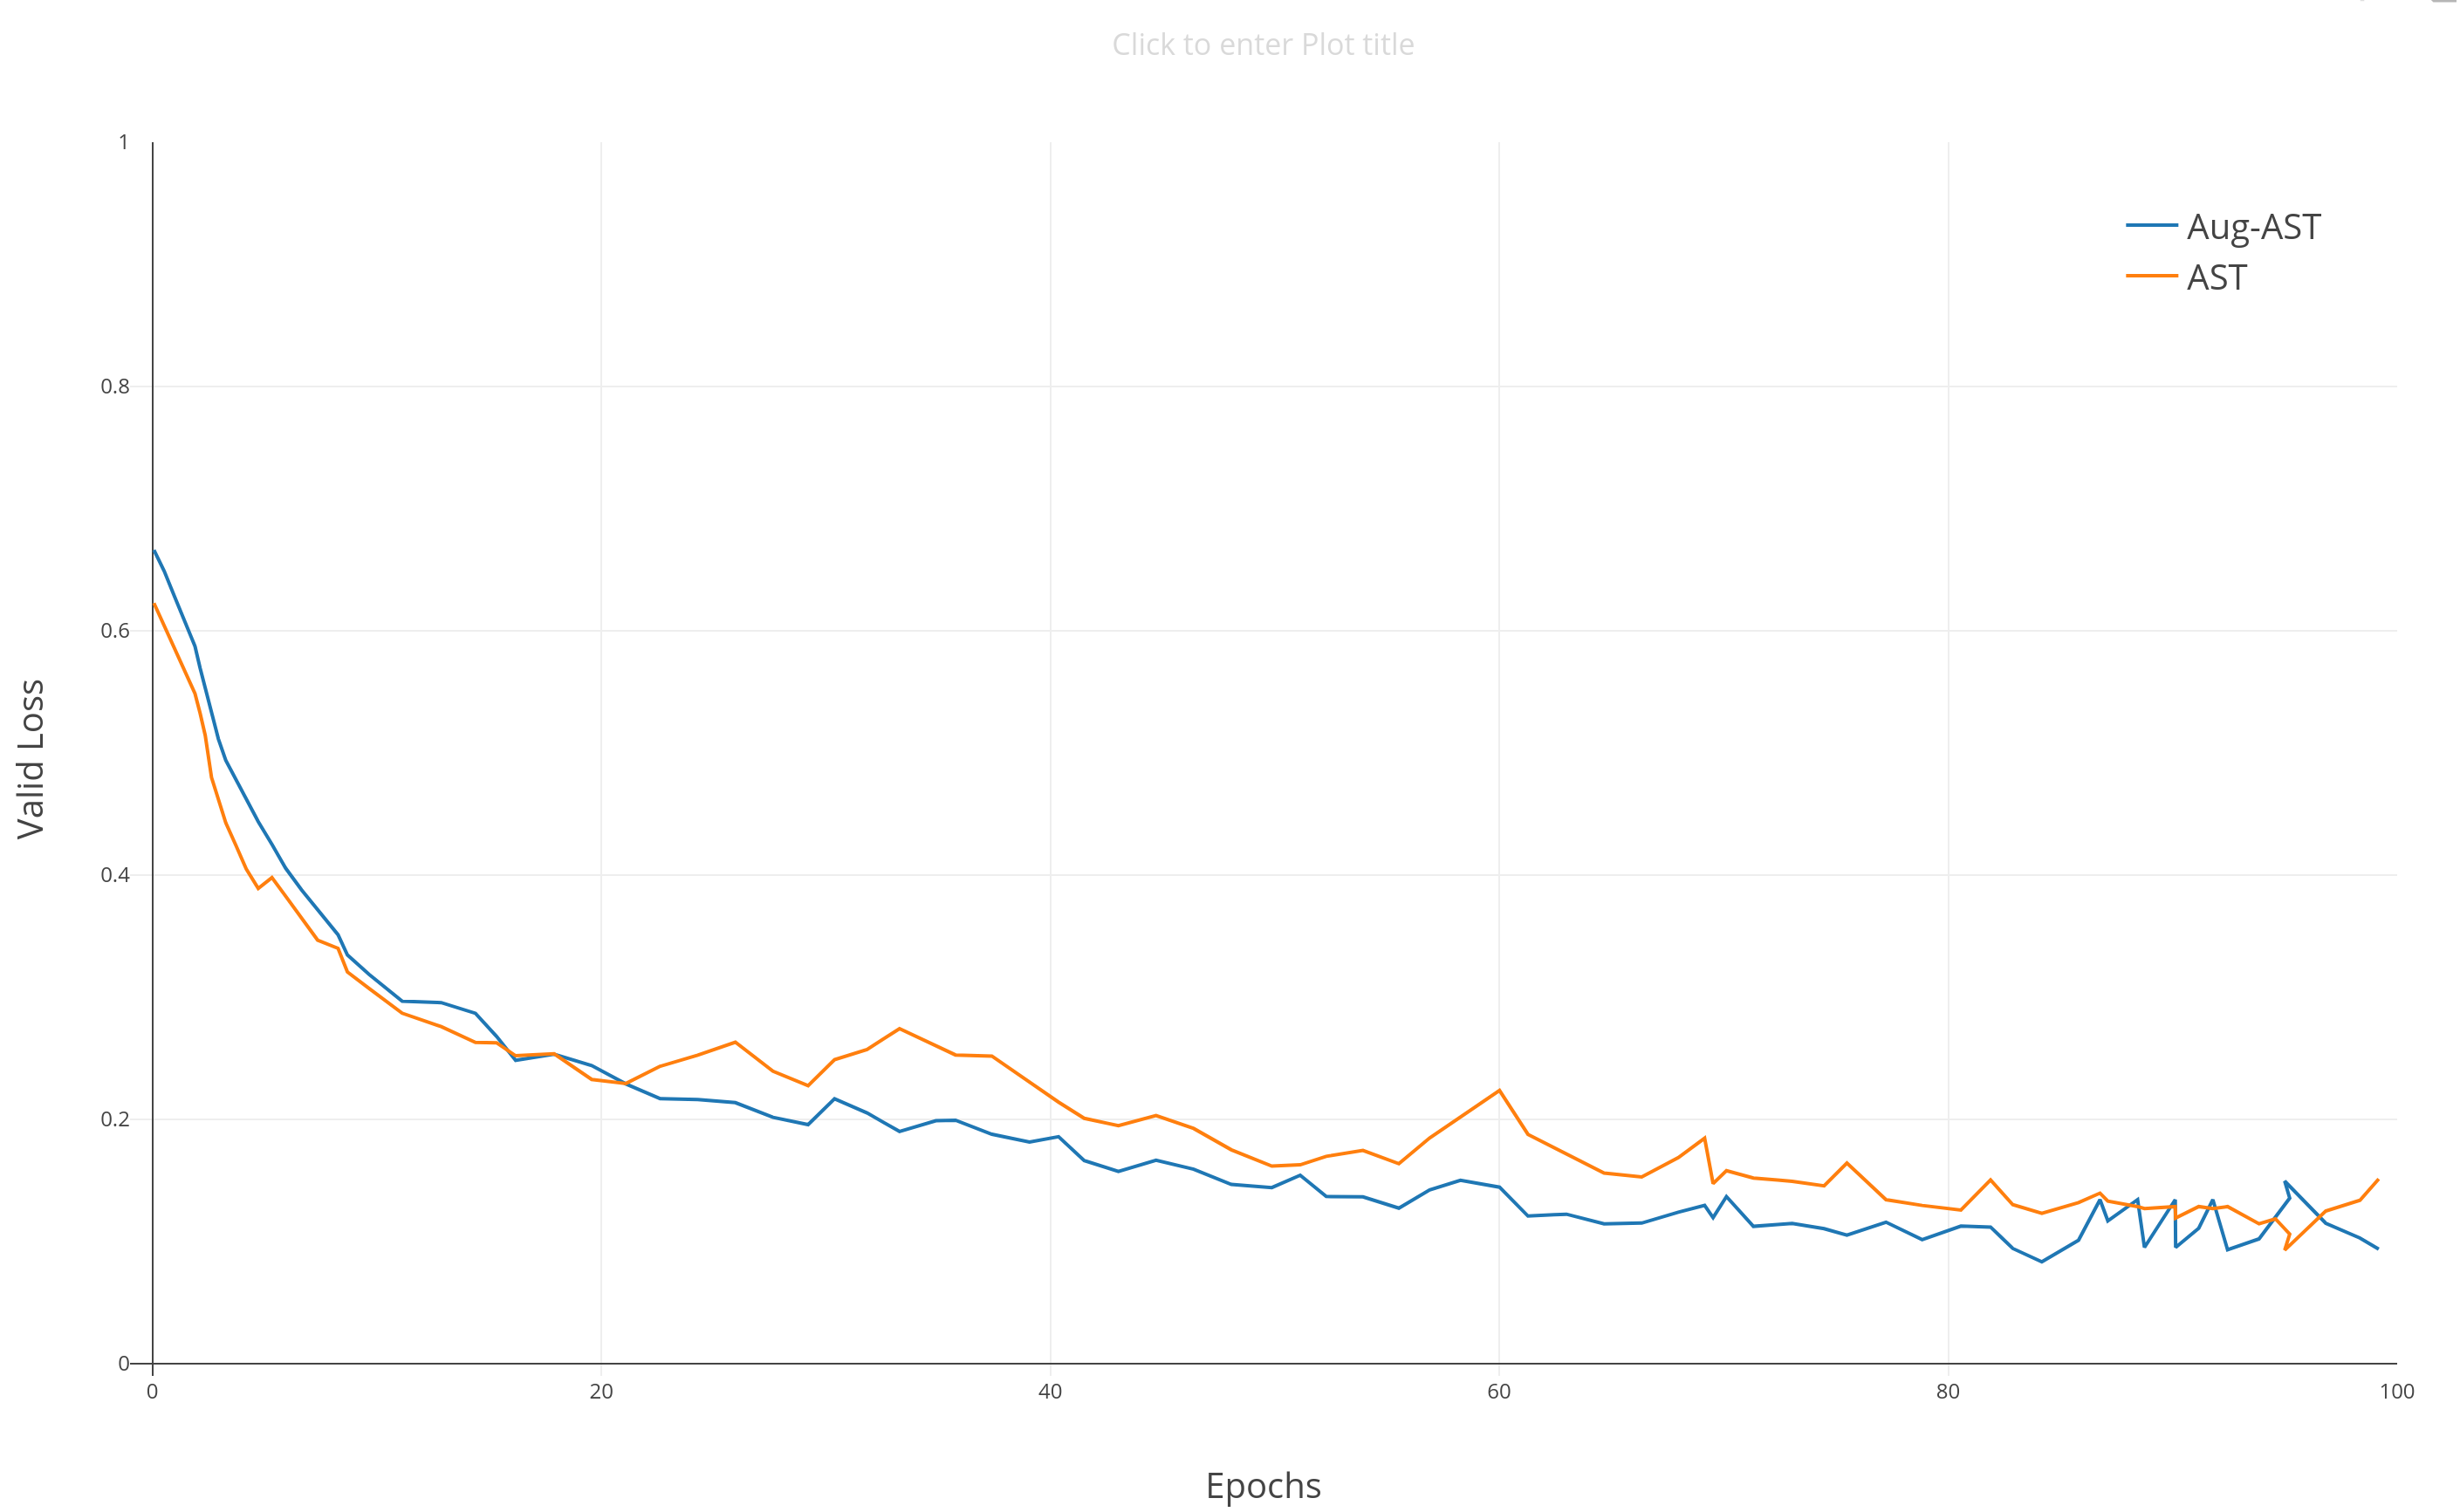}
    \caption{Average validation loss for AST and Aug-AST representation.}
    \label{fig:ast_loss}
\end{figure}

\begin{figure}[h]
    \centering
    \includegraphics[width=8cm]{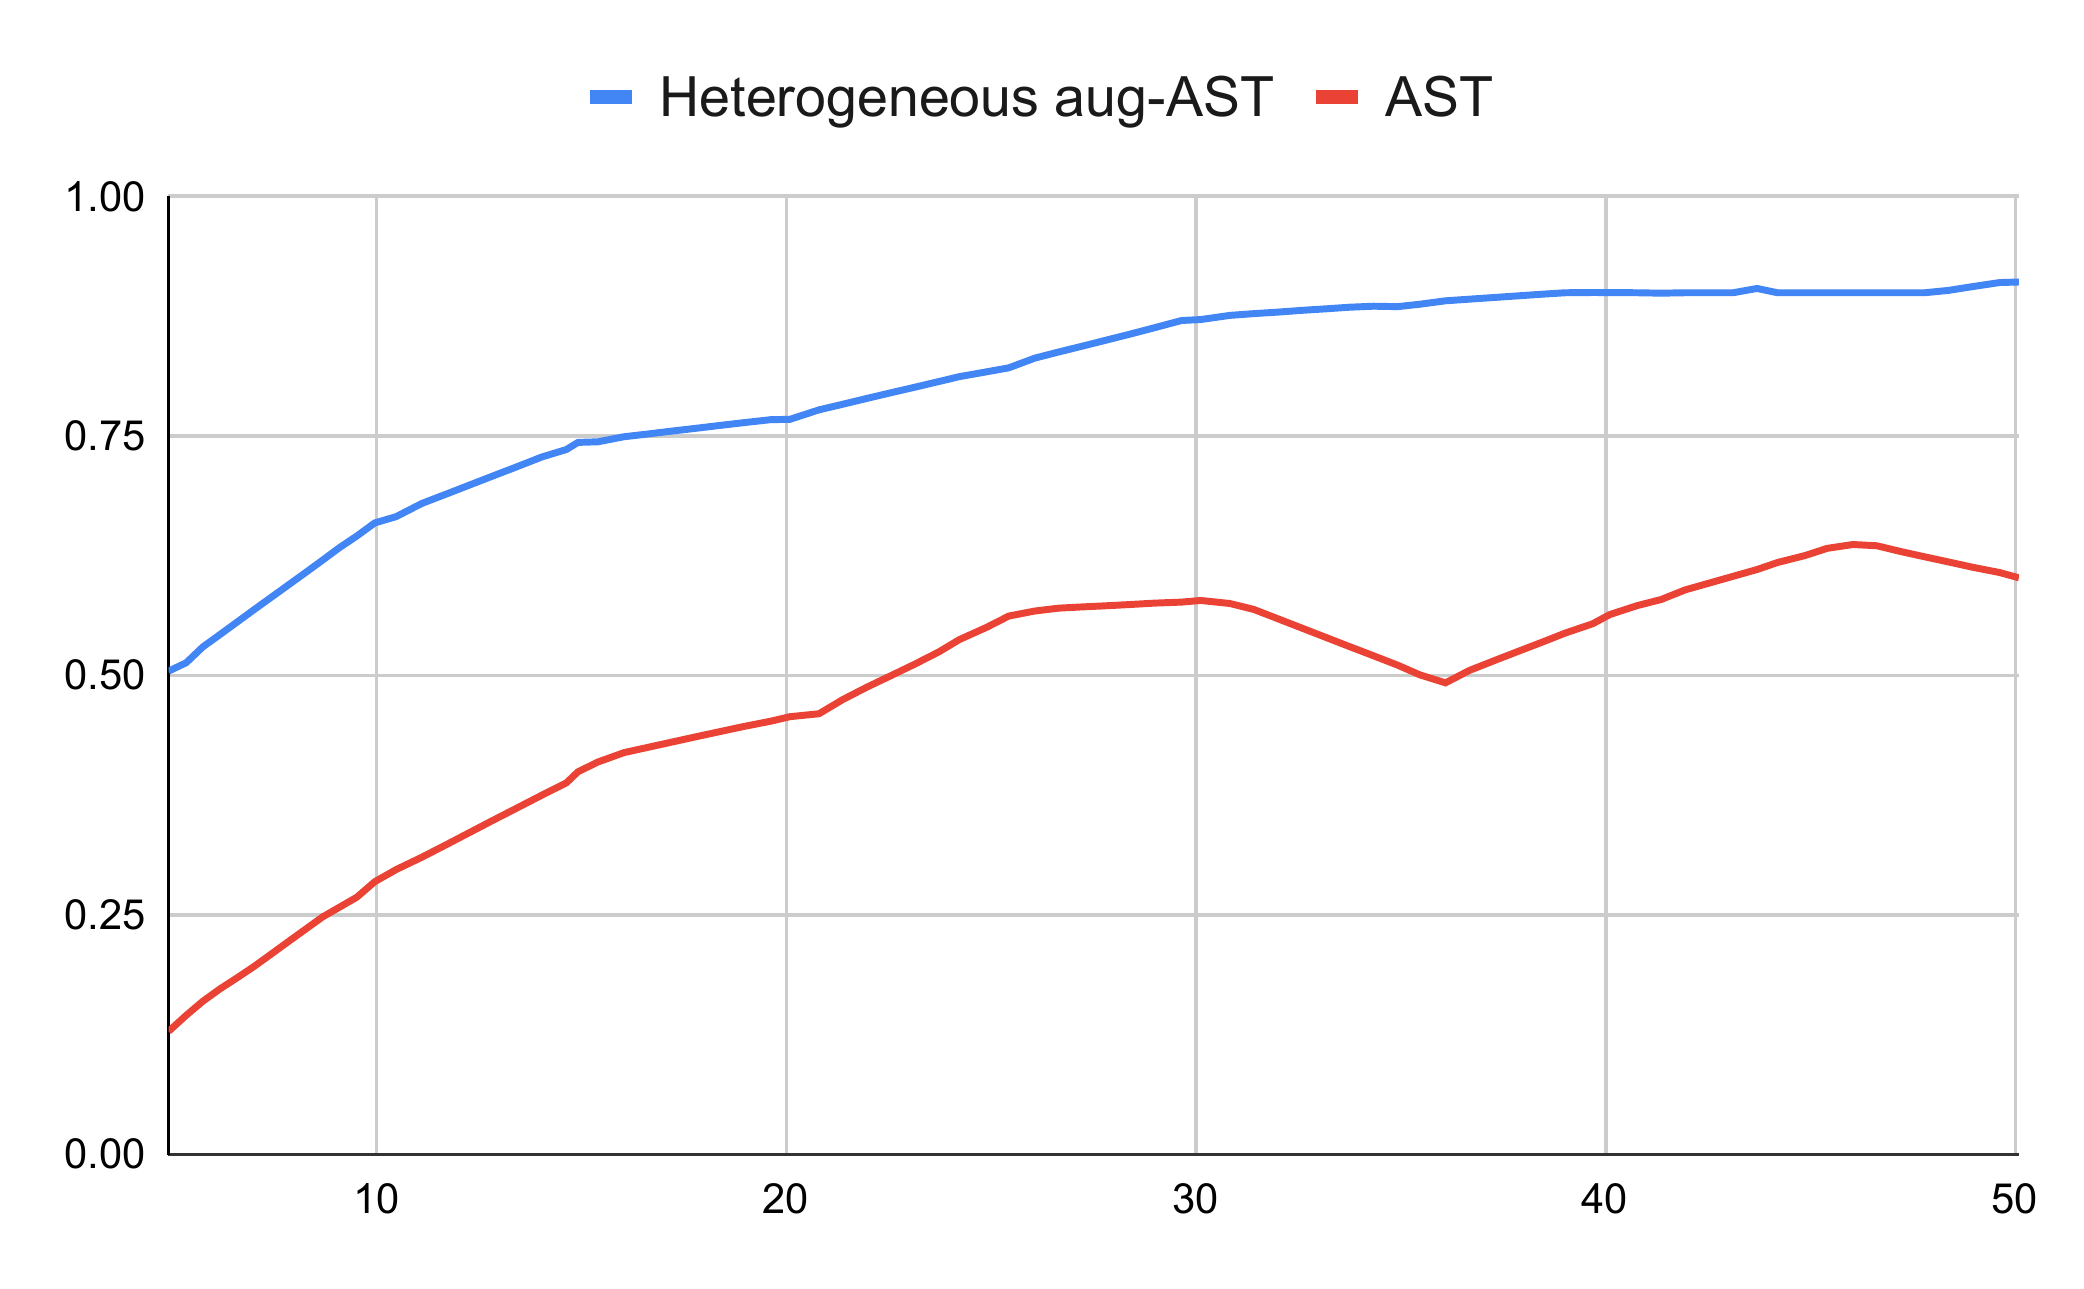}
    \caption{Accuracy of Heterogeneous aug-AST and Aug-AST representation.}
    \label{fig:acc}
\end{figure}

\begin{figure}[h]
    \centering
    \includegraphics[width=8cm]{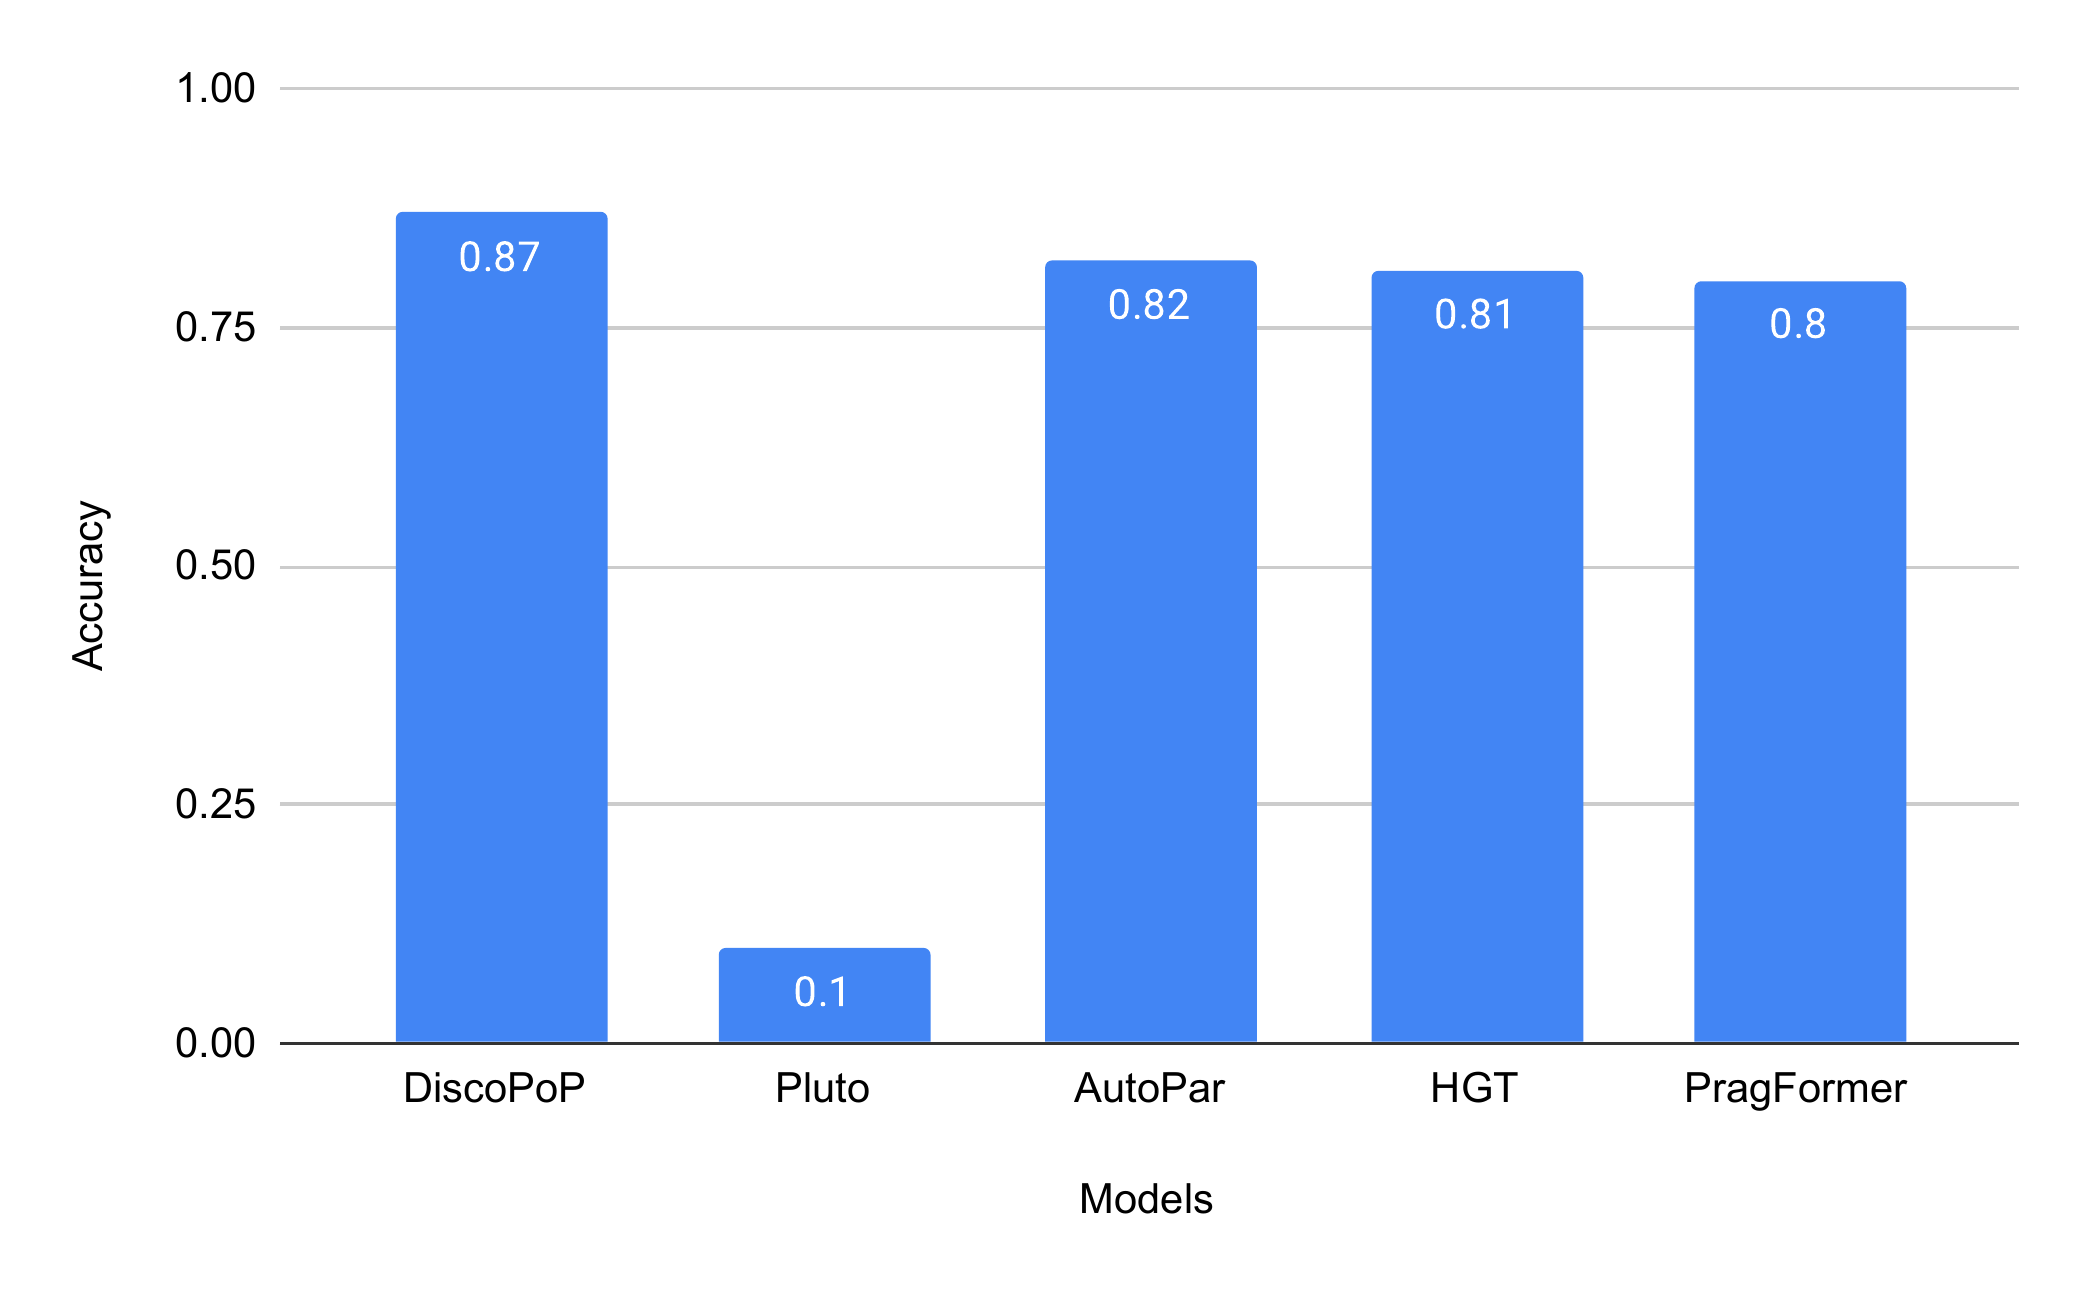}
    \caption{Accuracy of identifying the need for an OpenMP directive.}
    \label{fig:acc2}
\end{figure}
